# Supplementary material for: Debiasing Multimodal Sarcasm Detection with Contrastive Learning
Source: arXiv:2312.10493 source file (2023-12-19)
Supplement: Supplementary file 1 [file Appendix.tex]

\begin{appendices}

% \section*{Appendix}
\appendix
% \clearpage

\begin{figure*}[htbp!]
    \centering
    \includegraphics[width=0.93\linewidth]{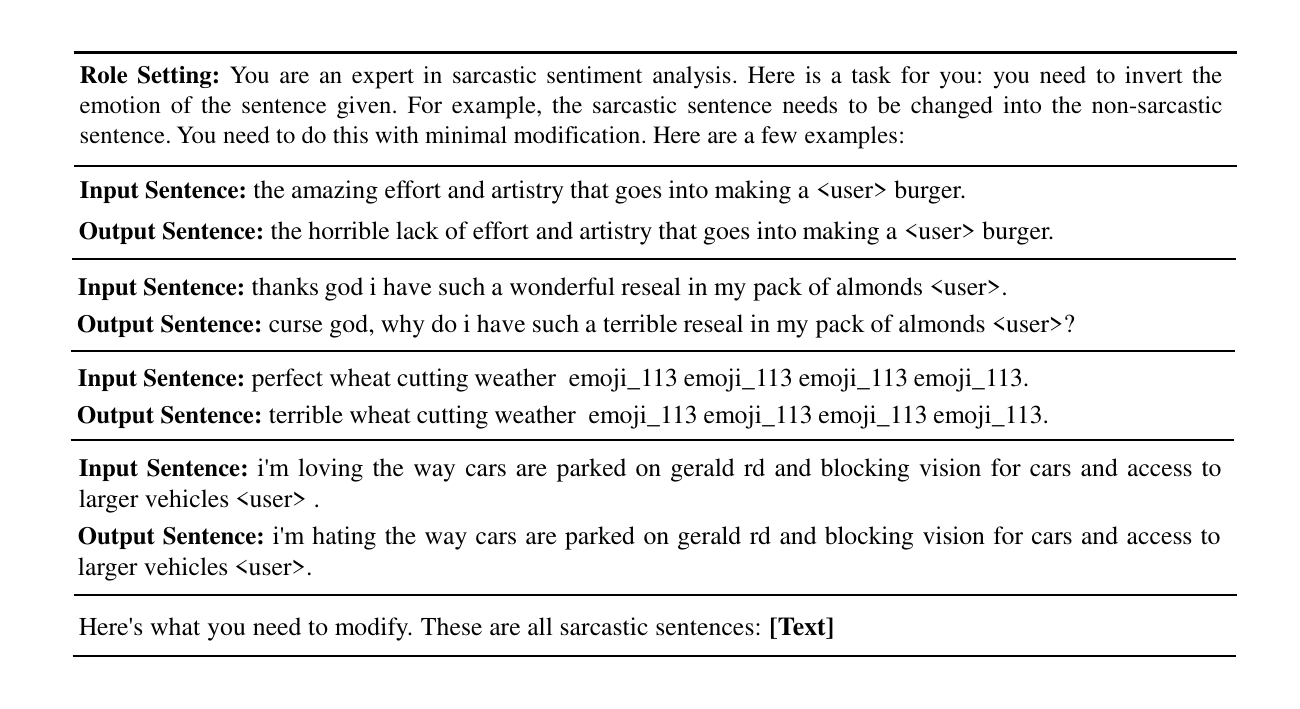}
    \vspace{-2em}
    \caption{Illustration of prompt for generating emotion-aware sarcastic sample.}
    \label{fig:enter-label1}
\end{figure*}

\begin{figure*}[h!]
    \centering
    \includegraphics[width=0.85\linewidth]{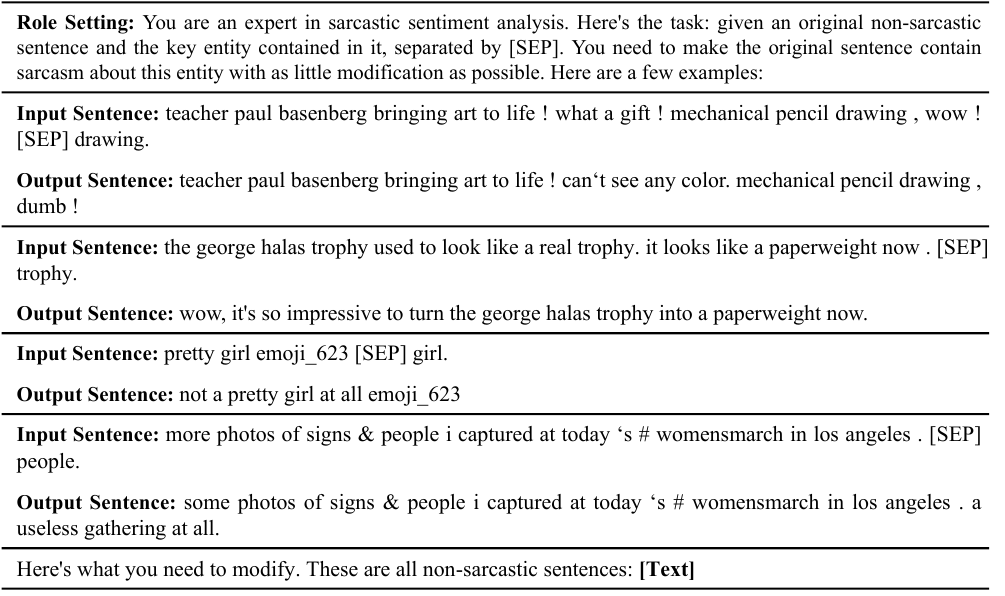}
    \caption{Illustration of prompt for generating entity-driven non-sarcastic sample.}
    \label{fig:enter-label}
\end{figure*}

\clearpage
\end{appendices}
